# Supplementary material for: Plasticity and evolvability under environmental variability: the joint role of fitness-based selection and niche-limited competition
Source: arXiv:2202.08834 source file (2022-07-06)
Supplement: Supplementary file 1 [file appendix.tex]

\onecolumn
\section{Appendix}

\subsection{Algorithm}
We present the pseudocode describing how evolution takes place in Algorithm \ref{alg:evolution}, which contains the initialization of the population and environment (Lines 2-8) and their updates at each generation based on the climate function $L$, and Algorithm \ref{alg:reproduce}, which provides more details on how reproduction differs depending on the selection mechanism.

\begin{algorithm}
\caption{evolution}
\label{alg:evolution}
\begin{algorithmic}[1]
\State \textbf{Input:} $\mathcal{K},\mathcal{N},\mathcal{G},\epsilon,L,C_{\text{ref}},S$

\State $\mathcal{K}$.initializeGenomes()

\State $e_0^0=L(0)$
\State $\mathcal{N}$.initializeNiches($ C_{\text{ref}}, e_0^0, \epsilon$ )

\For{$g  \in \mathcal{G}$}

    \State $e_0^g=L(g)$ \Comment{Climate function transitions}

    \State $\mathcal{N}$.updateNiches($ C_{\text{ref}}, e_0^g$ ) \Comment{Update environmental state of all niches based on new climate}

    \State $\mathcal{K}$.reproduce($\mathcal{N},S,g$)
\EndFor
\end{algorithmic}
\end{algorithm}
\begin{algorithm}
\caption{reproduce}
\label{alg:reproduce}
\begin{algorithmic}[1]
\State \textbf{Input:} $\mathcal{K}, \mathcal{N}, S, g$ \Comment{$S\in \{\{N\}, \{F\}, \{N,F\}\}$}
\State 
\If{$N\in S$} \Comment{Niche-limited competition}
    \State $\text{population} = \{\mathcal{K}.\text{survive}(n)~|~ n\in \mathcal{N}\}$ \Comment{See Eq~\ref{eq:survive_niche}}
    \State $\text{capacity} = \{c_n^g~|~n\in \mathcal{N}\}$ \Comment{See Section~\ref{sec:env_model}}
\Else \Comment{Only fitness-based selection}
    \State $\text{population} = \{\mathcal{K}\}$ \Comment{no niche-limited competition, see Section~\ref{sec:select_mechanism}}
    \State $\text{capacity} = \{\sum_{n\in \mathcal{N}} c_n^g\}$
\EndIf

\If{$F\in S$} \Comment{Fitness-based competition}
\State select="fitness-based" \Comment{Selection of the fittest}
\State population.order() \Comment{Order the population of each niche based on fitness}
\Else \Comment{No fitness-based competition}
\State select="random" \Comment{Random selection}
\EndIf
\State 
\For{$\text{p, c} \in \text{zip(population, capacity)}$} \Comment{For each population with its own capacity}
\State $size=0$
\While{$\text{size} < c$}
\State p = p[:capacity] \Comment{Drop agents that do not fit in the niche}
\State offspring = p.mate(select) \Comment{See Section~\ref{sec:select_mechanism}}
\State offspring.mutate() \Comment{Eq~\ref{eq:mutation}}
\State $\text{size} \gets \text{size} + 1$
\EndWhile
\EndFor

% \If{S $==$ F-selection}
%     \State K.rank()
%     \State $K^{'} = \{ \}$ 
%     \While{$K^{'} < c_{\text{total}}$}
%         \State offspring=k.mate(prob=k.fitness)
%         \State offspring.mutate()
%         \State $K^{'}$.append(offspring)
%     \EndWhile
% \EndIf
% \If{S $==$ N-selection or S $==$ NF-selection}
%     \For{$n \in \{1, \ldots, N\} $}
%     \State $K_n$ = K.survive(n)
%     \If{S $==$ F-selection}
%          \State $K_n$.rank()
%     \Else
%         \State $K_n$.shuffle()
%     \EndIf
%     \State $K^{'}_n = \{ \}$ 
%     \While{$K^{'}_n < c_{n}$}
%         \If{S $==$ NF-selection}
%              \State offspring=k.mate(prob=k.fitness)
%         \Else
%             \State offspring=k.mate(prob=1)
%         \EndIf
        
%         \State offspring.mutate()
%         \State $K^{'}_n$.append(offspring)
%     \EndWhile
%     \EndFor
% \EndIf
\end{algorithmic}
\end{algorithm}

\subsection{Notation}
This section contains a summary of the notation used throughout the paper in Table \ref{tab:notation}.

\begin{table}
\begin{center}
\begin{adjustbox}{max width=\textwidth}
\begin{tabular}{ |l|l|l| } 
 \hline
 Population & Environment & Evaluation \\ 
 \hline
 $K$, population size & $L: \mathcal{G} \rightarrow R$, climate function & $\bar{mu}^g$, population-average ideal environmental state \\ 
 $\mu_k^g$, mean of tolerance curve  & $N$, number of niches & $\bar{\sigma}^g$, , population-average plasticity \\ 
 $\sigma_k^g$, standard deviation of tolerance curve  &  $e_0^g=L(g)$, reference environmental state &  $\bar{\sigma}^g$, population-average evolvability \\
 $r_k^g$, mutation rate  & $e_n^g=e_0^g + 0.01 n$, environmental state & \\
 $o_k^g=[\mu_k^g, \sigma_k^g, r_k^g]$, genome  & $C_{\text{ref}}=K_{\text{max}}$, reference capacity & $X^g$, extinction events \\
 $O \in [O_{\text{evolve}},O_{\text{no-evolve}}]$, genome evolution model  & $C_N=C_{\text{ref}}/N$ climate-independent capacity & \\
    & $c_n^g=e_n^g \cdot C)N$ climate-dependent capacity & $D$, dispersal (see Section \ref{sec:eval_metrics} for definition)\\
& $S \in [\text{F-selection, N-selection, NF-selection}]$, selection mechanism & $V^g=\sigma_{\mu_g} + \sigma_{\sigma_g} +  \sigma_{r_g}$, (genotypic) diversity \\
 & $\epsilon$, vertical offset between adjacent niches & $A$, survival indicator\\ 
  \hline
\end{tabular}
\end{adjustbox}
\end{center}
\caption{Notation used to indicate features of the population, environment and evaluation metrics: Super-script $g \in \mathcal{G}=\{1, \cdots, G\}$ is the generation index, while sub-scripts $k \in \mathcal{K}=\{1, \cdots, K\}$ and $n \in \mathcal{N}=\{1, \cdots, N \}$ are indexes for individuals and niches respectively.}
\label{tab:notation}
\end{table}
